# Supplementary material for: Mapping Firms' Locations in Technological Space: A Topological Analysis of Patent Statistics
Source: arXiv:1909.00257 source file (2022-03-31)
Supplement: Supplementary file 1 [file x_old_appendix.tex]

\clearpage
\pagenumbering{arabic} \renewcommand*{\thepage}{A-\arabic{page}} \appendix 
%\singlespacing

\section*{Appendix (For Online Publication)}

\subsection*{B. \ Proofs and Computations}

\subsection*{C. \ Additional Figures and Tables for Sections 4, 5, and 6}

\clearpage

\subsection*{D. \ Additional Descriptions of the Mapper Graphs}

This section provides additional descriptions of the Mapper graphs in sections 4 and 6.

\subsubsection*{D.1 \ Supplementary Descriptions of the Mapper Graph in Section 4}

\paragraph{\protect IT} Some of the big names are extremely unique, thus forming their own ``islands,'' or smaller connected components that are isolated from the continent. For example, IBM had no peers in the 1970s--1990s (see its small island in the upper-middle part). Its R\&D activities were massive, diverse, and different from any other firm's. Its restructuring in the early 2000s made it somewhat comparable to HP, as suggested by their rendezvous at the end of HP's flare (see the top-left part).\footnote{Flares reflect continuous changes over time. Sudden jumps, such as the disconnection within IBM between the 1990s and the 2000s, tend to occur when firms go through major corporate reorganization.} 

Other global brands display surprisingly short flares, for multiple reasons. Consumers might perceive Apple's products as innovative, but their main appeal is design and functionality, which do not necessarily represent patentable inventions. Most software/internet firms (e.g., Google, Adobe, and eBay) were relatively new during the sample period and did not have time to develop unique patent portfolios.

Another curious case is Cisco and Microsoft, both of which heavily patented in classes 370 and 709 in the late 1990s.\footnote{USPTO class 370 is ``multiplex communications'' and class 709 is ``electrical computers and digital processing systems: multicomputer data transferring.''} Their substantial overlap connects the two flares in the middle, without which they would have looked separate and longer. This example highlights an important aspect of our analysis: uniqueness is a relative concept. That is, a firm's flare length is determined by not only its own patenting patterns, but also all other firms' trajectories, because it is based on the entire graph.

\paragraph{\protect Pharmaceuticals and Chemicals} Monsanto, an agrochemical firm, appears in another flare that connects with drug makers. However, a closer look into its time path reveals the flare is moving \textit{inward}, rather than outward as in the case of most other firms. Its patents in the 1970s and the 1980s are mostly unrelated to drugs, but those in the 1990s and the 2000s are in areas in which drug makers patent. Monsanto is one of the few centripetal flares in the graph, which suggests the firm employed highly idiosyncratic R\&D strategies.

Finally, conglomerates in general chemistry (Dow, DuPont, and 3M) form their own long flares at the southern end of the continent. This pattern is reminiscent of the engineering conglomerates' island in Figure \ref{Figure - mapper(cos_log_details)} (b). The ability to capture and visualize the relative proximity of conglomerates appears to be a unique strength of our approach, because their entire business portfolios are often too large and complicated to study otherwise (e.g., by using conventional IO methods at the individual product-market level).

\paragraph{\protect Patents Acquired by M\&As} Computers, semiconductors, and telecommunications firms now form ``super flares'' that contain multiple firms in the same industries, respectively, rather than individually spiking out from the main trunk. Even IBM, whose patents in the 1970s--1990s form an island in the previous graph, is now part of the computer super flare. Likewise, whereas AT\&T and other large telecommunications firms form their own island in Figures \ref{Figure - mapper(n20_m0_cos)} and \ref{Figure - mapper(cos_log_details)}, this telecom island becomes a ``peninsula'' in Figure \ref{Figure - mapper(cos_log_m2)} and is connected to the main continent via Nokia's flare. The manufacturers of semiconductor devices (e.g., Intel, Texas Instruments, and LSI Logic) form another super flare as well.

Aerospace and engineering firms go even further and form a ``loop'' instead of individual flares or super flares. That is, their extended (R\&D + M\&A) patent portfolios connect with the main trunk at multiple points. This pattern suggests these firms operate in a continuum of technological areas that relate to multiple different sectors.

\subsubsection*{D.2 \ Supplementary Descriptions of the Mapper Graph in Section 6}

\subsection*{E. \ Additional Literature Review}

This section provides an additional literature review.

For surveys and examples of the literature that introduces novel techniques from mathematics, statistics, and computer science to analyze high-dimensional data to economics, see \cite{belloni2014high}, \cite{varian2014big}, \cite{athey2017state}, \cite{brumm2017using}, \cite{ChernozhukovEtAl2018ECTJ}, \cite{cattaneo2019two}, \cite{gentzkow2019text}, \cite{IskhakovRustSchjerning2020}, and \cite{Igami2020}.

Even though this is the first paper to use TDA and the Mapper algorithm \textit{in economics} to our knowledge, we are aware of several applications of TDA to financial time series (\cite{Gidea2017}, \cite{GIDEA2018820}, \cite{GUO2020124956}, \cite{GOEL2020113222}, \cite{MAJUMDAR2020113868}, \cite{QIU2020113475}). However, they are relatively short papers primarily by non-economists and published in either computer science or physics journals, with limited connections to economics.

For the well-known limitations of patent statistics, see, for example, Griliches (1990), Lerner and Seru (2017), and Igami and Subrahmanyam (2019).

Recent micro-econometric publications at top economics journals that use patents include \cite{cockburn2016patents}, \cite{howell2017financing}, \cite{AzoulayEtAl2019}, and \cite{sampat2019patents}, among many others. A major data-cleaning project is undertaken by \cite{AroraBelenzonSheer2019}, who extend the NBER patent database of \cite{hall2001nber} and \cite{bessen2009nber} to 2015, linking firm names to the Compustat financial data. Since December 2019, such efforts to construct and improve patent-based innovation metrics have been renewed and coordinated under the \textit{NBER Innovation Information Initiative} organized by Adam Jaffe.

An additional example of the use of text analysis in IO is \cite{hoberg2016text}, which use text analysis on firms' Form 10-K product descriptions to describe and characterize product-market competition.

%%% Local Variables:
%%% mode: latex
%%% TeX-master: "TDAPatent"
%%% End:
